# Supplementary material for: C$\cdot$ASE: Learning Conditional Adversarial Skill Embeddings for Physics-based Characters
Source: arXiv:2309.11351 source file (2023-09-20)
Supplement: Supplementary file 1 [file supp.tex]

\documentclass[acmtog,anonymous,review]{acmart}

% Added pkgs
\usepackage{arydshln}
\usepackage{multirow}
\usepackage{threeparttable}
\usepackage[percent]{overpic}
\usepackage{arydshln}
\usepackage{booktabs}
\usepackage{amsmath}
\usepackage{xspace}
\usepackage{wrapfig}
\usepackage[ruled]{algorithm2e}

%% Rights management information.  This information is sent to you
%% when you complete the rights form.  These commands have SAMPLE
%% values in them; it is your responsibility as an author to replace
%% the commands and values with those provided to you when you
%% complete the rights form.
%\setcopyright{acmcopyright}
%\copyrightyear{2018}
%\acmYear{2018}
%\acmDOI{XXXXXXX.XXXXXXX}

%%
%% These commands are for a JOURNAL article.
\acmJournal{TOG}
%\acmVolume{37}
%\acmNumber{4}
%\acmArticle{111}
%\acmMonth{8}

%%
%% Submission ID.
%% Use this when submitting an article to a sponsored event. You'll
%% receive a unique submission ID from the organizers
%% of the event, and this ID should be used as the parameter to this command.
\acmSubmissionID{619}

%%
%% The majority of ACM publications use numbered citations and
%% references.  The command \citestyle{authoryear} switches to the
%% "author year" style.
%%
%% If you are preparing content for an event
%% sponsored by ACM SIGGRAPH, you must use the "author year" style of
%% citations and references.
\citestyle{acmauthoryear}

\newcommand{\name}{E$\cdot$ASE\xspace}

\begin{document}
%\title[Condition Motion GAN]{\name: Conditional Adversarial Skill Embeddings for Elite Physics-based Characters}
%\title[Condition Motion GAN]{ASE-Elite: Conditional Adversarial Skill Embedding for Physics-based Character Control}
\title{Supplementary material: \\
\name: Learning Conditional Adversarial Skill Embeddings for Elite Physics-based Characters}
%\name: Elite Physics-based Characters with Conditional Adversarial Skill Embeddings

%% Authors
\author{First Author}
\email{firstauthor@example.com}
\orcid{1234-5678-9012}
\affiliation{%
  \institution{First Institution}
  \country{Firstcountry}
}

\author{Second Author}
\orcid{1234-5678-9012}
\affiliation{%
  \institution{Second Institution}
  \country{Secondcountry}
}

\renewcommand{\shortauthors}{Firstauthor et al.}

\newcommand{\ZY}[1]{{\color{cyan}ZY:#1}}
\newcommand{\XL}[1]{{\color{blue}XL:#1}}
\newcommand{\QN}[1]{{\color{orange}QN:#1}}
\newcommand{\TODO}[1]{{\color{red}TODO:#1}}
\newcommand{\todo}[1]{{\color{red}todo:#1}}
\newcommand{\update}[1]{{\color{red}#1}}
\maketitle

%% import all math symbols
\input{math_utils}

%% The actual document with your content starts here
% \clearpage
\input{6-appendix}

%% Bibliography.
%% Uncomment the bibliography line and link to an actual bib file
\bibliographystyle{ACM-Reference-Format}
\bibliography{bibliography.bib}

\end{document}
